# Supplementary material for: VCBench: Benchmarking virtual cell models for in-the-wild perturbation response
Source: arXiv:2604.27646 source file (2026-11-23)
Supplement: Supplementary file 1 [file X_appendix.tex]

\appendix

\setcounter{figure}{0}

\begin{figure}[htbp]
    \centering
    \includegraphics[width=\textwidth]{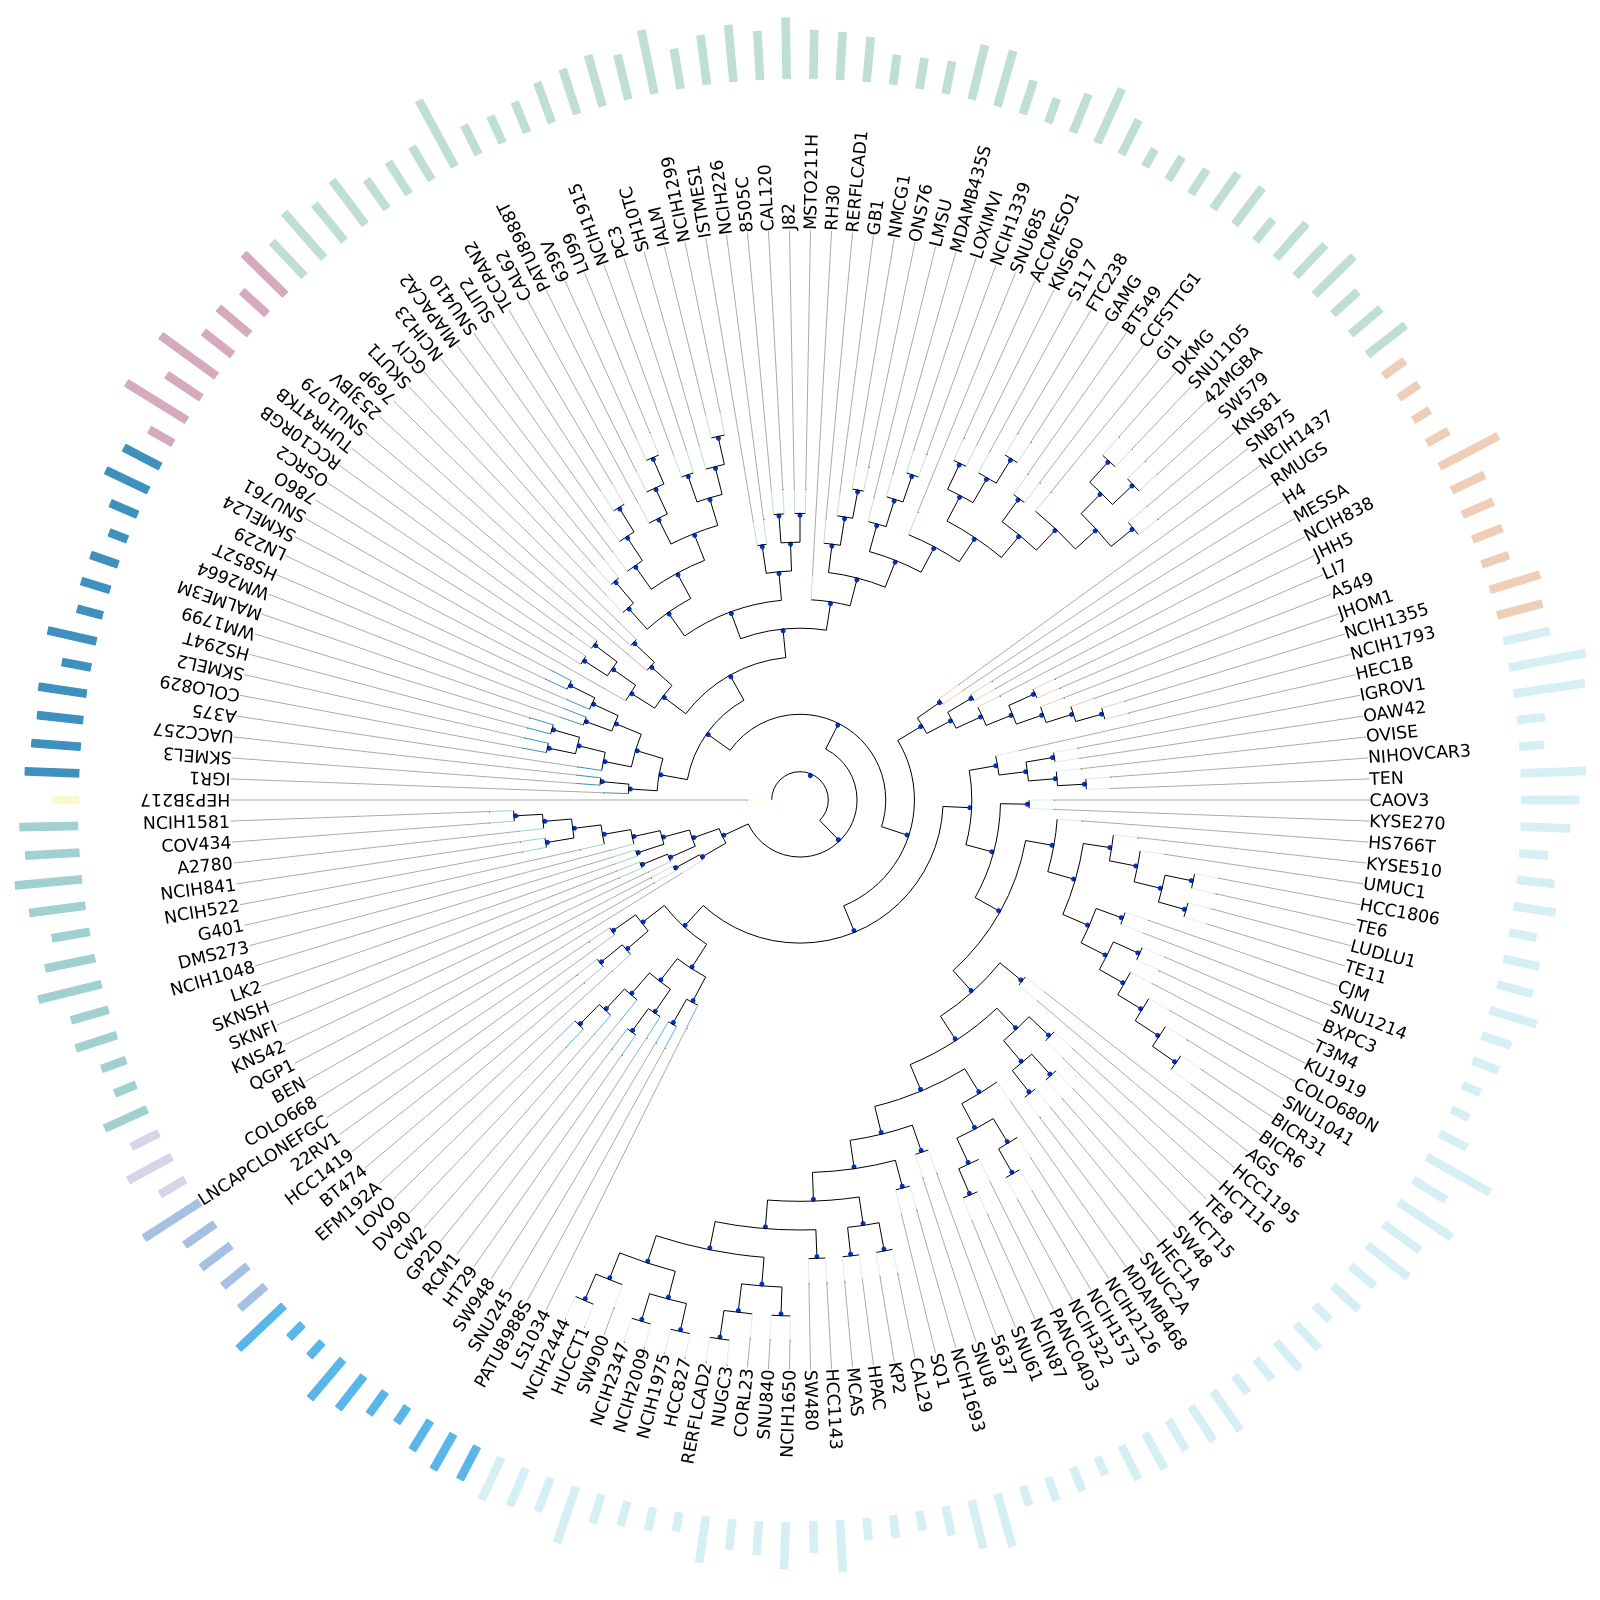}
    \caption{
    \textbf{Hierarchical clustering of cell lines based on STACK embeddings in the McFarland2020 dataset.}
    Cell lines are embedded using the STACK foundation model and clustered using cosine distance. The resulting hierarchy is partitioned into 10 meta-clusters, which are used to define cell-state-based splits for unseen-cell generalization.
    }
    \label{fig:stack_tree}
\end{figure}

\begin{figure}[htbp]
    \centering
    \includegraphics[width=\textwidth]{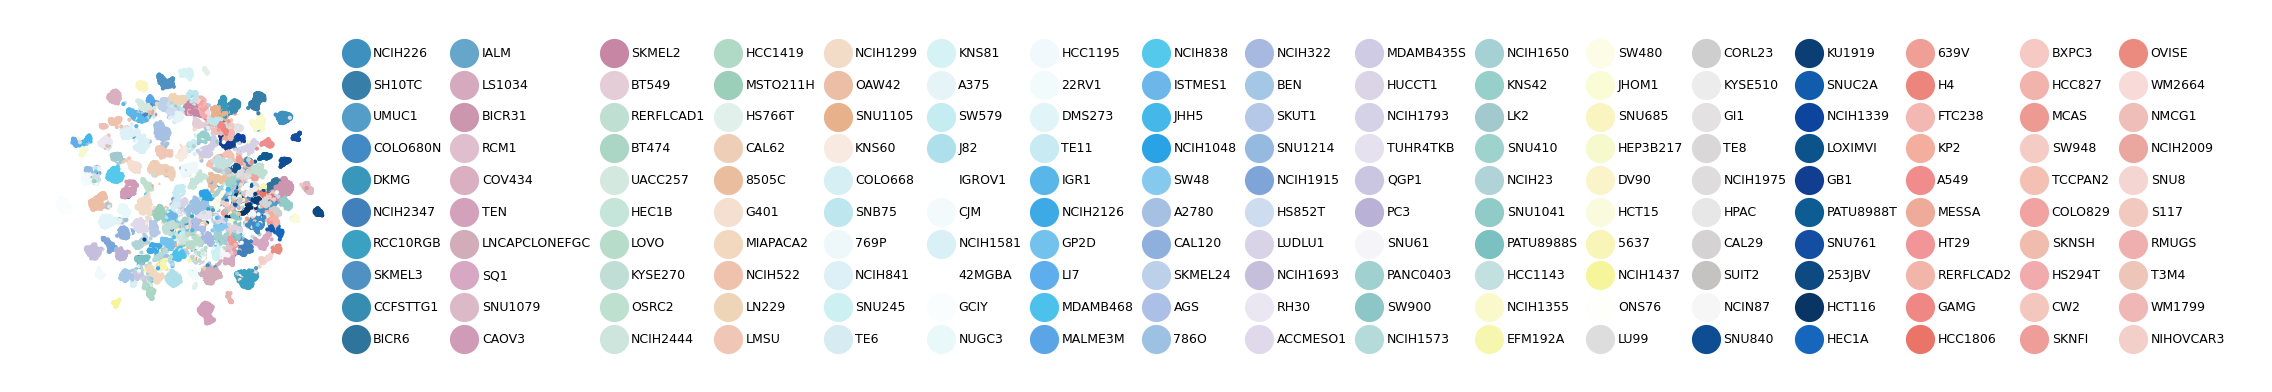}
    \caption{
    \textbf{Visualization of all cell line distribution in the McFarlandTsherniak2020 dataset.}
    UMAP projection of cells colored by cell line identity. Each point represents a single cell, and colors indicate distinct cell lines. 
    }
    \label{fig:umap_full_cellline}
\end{figure}

\begin{figure}[htbp]
    \centering
    \includegraphics[width=\textwidth]{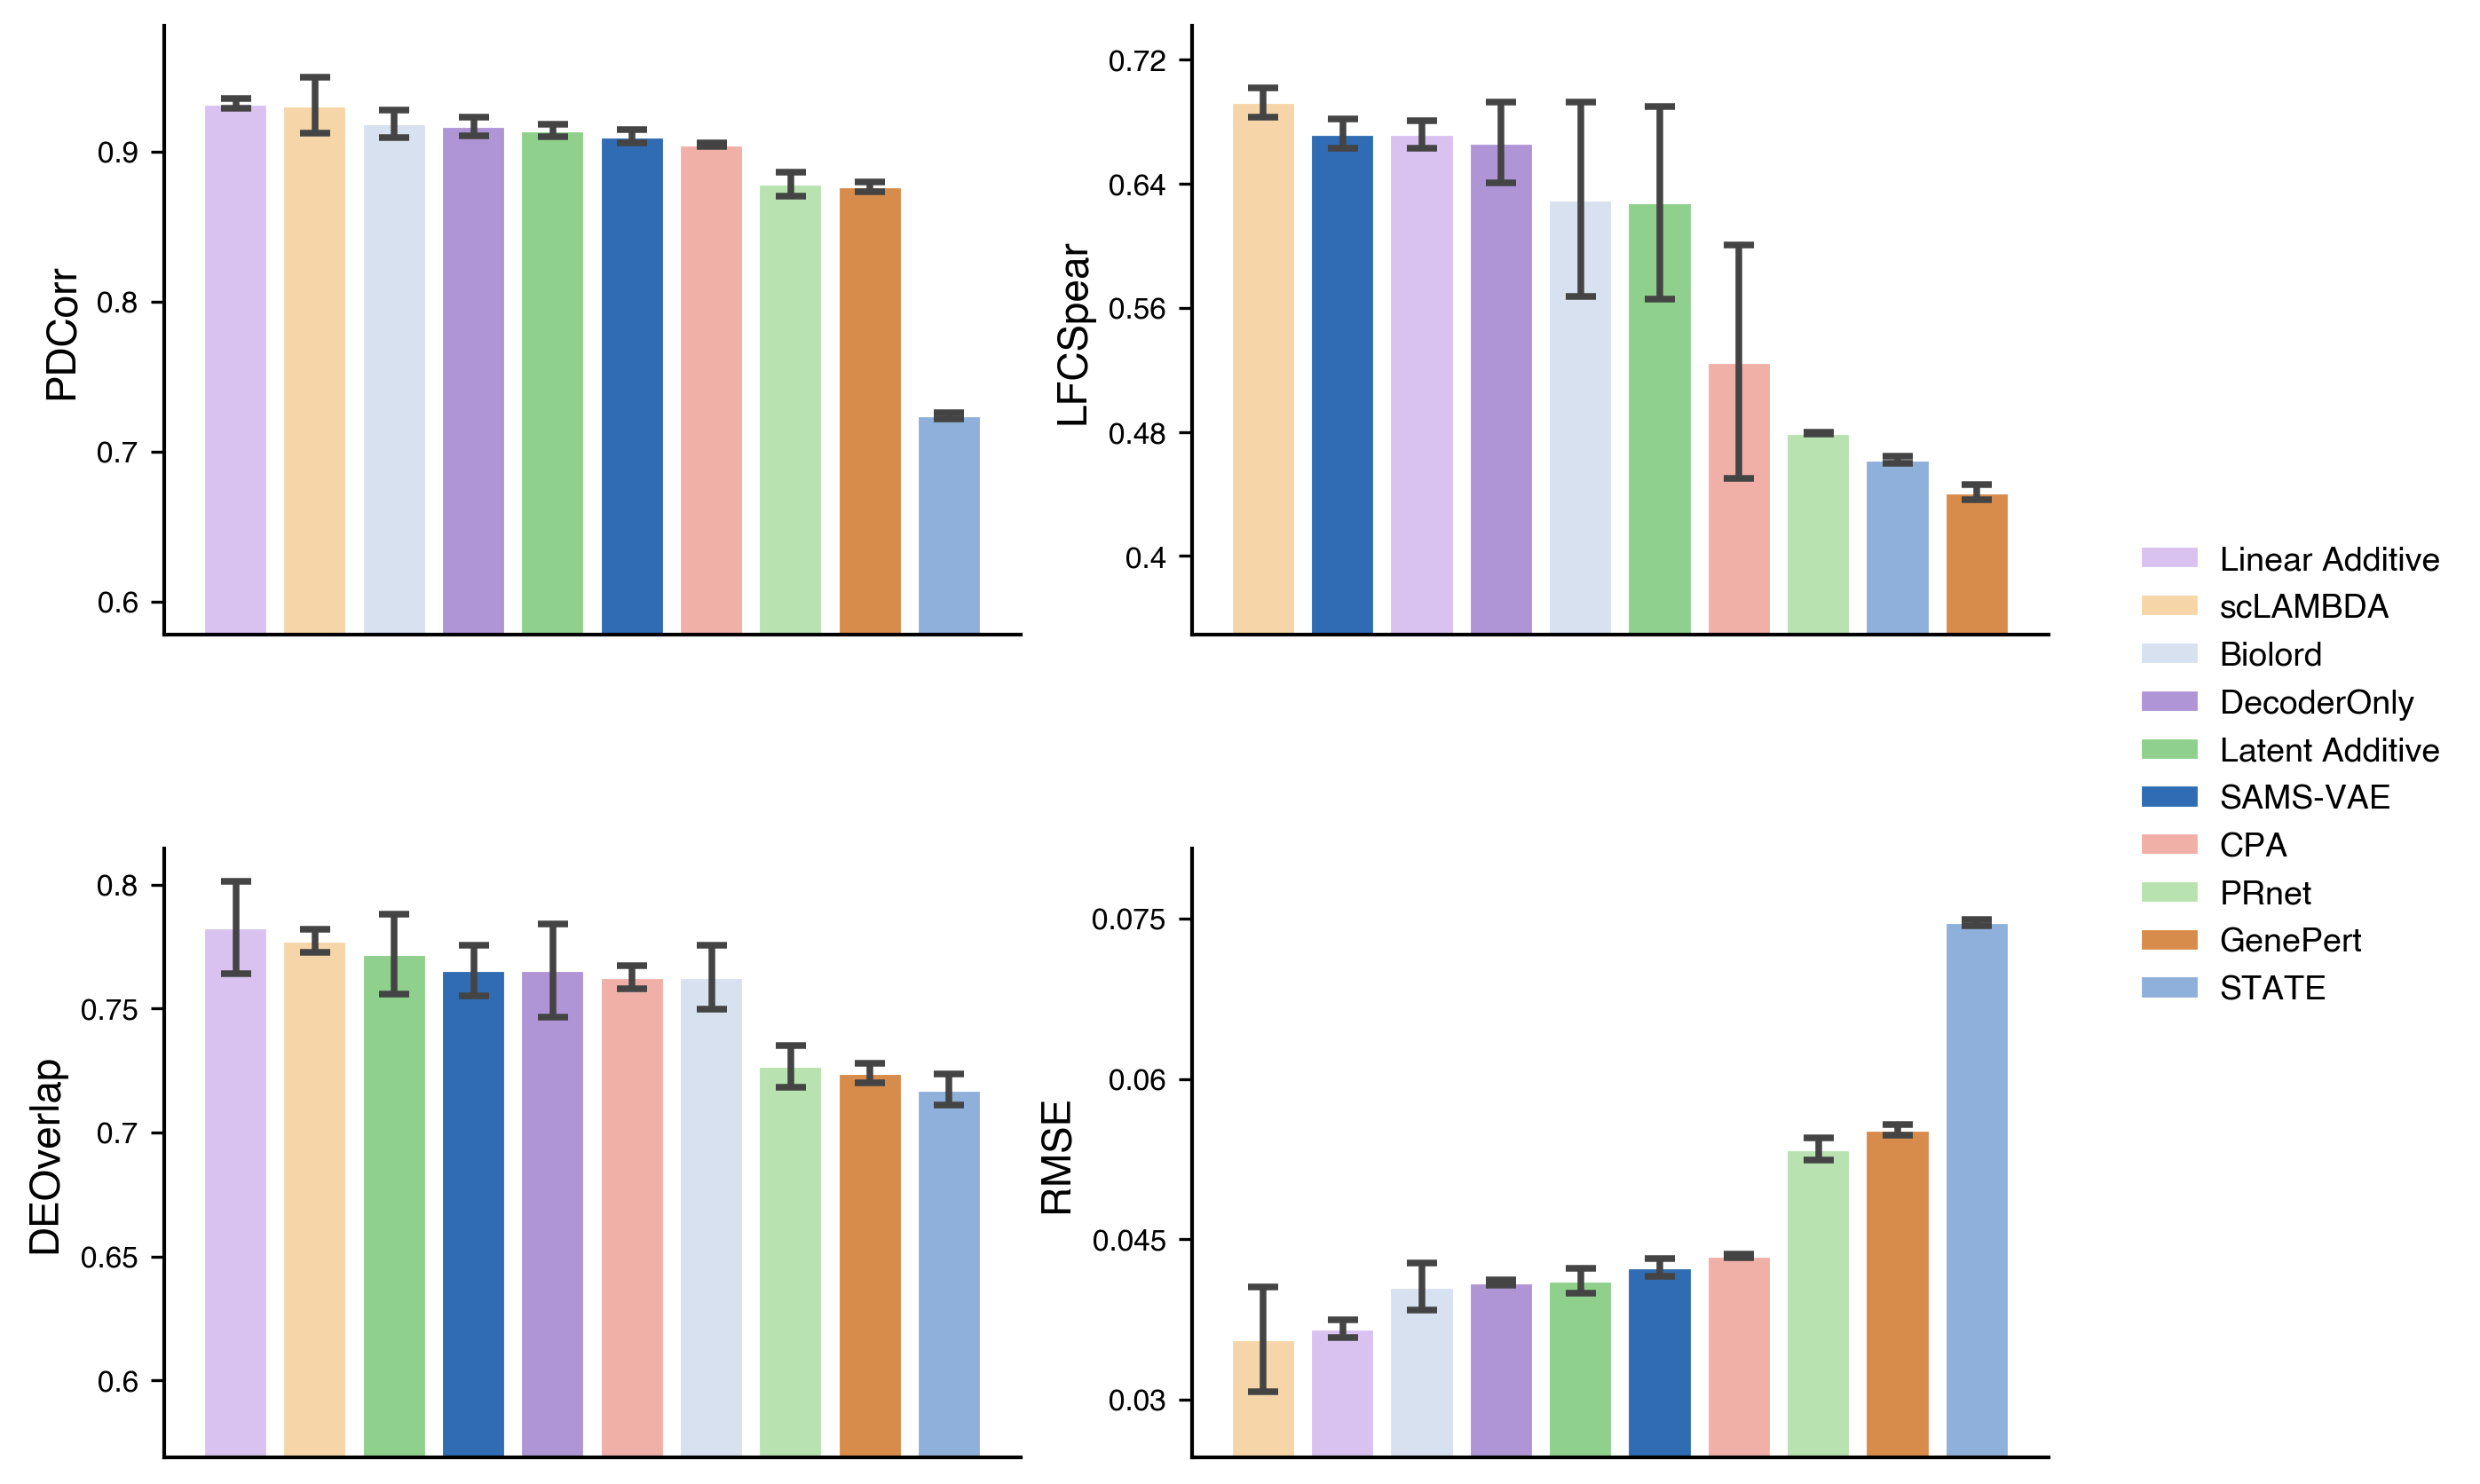}
    \caption{
    \textbf{Performance comparison of perturbation prediction models on the Kang2018 dataset without cell embedding.}
    Results are evaluated using four metrics: $\Delta$PCC, Spearman correlation of log fold change, DEG overlap, and RMSE. Each bar represents the mean performance across runs, and error bars indicate standard deviation. 
    }
    \label{fig:kang_noemb_metrics}
\end{figure}

\begin{figure}[htbp]
    \centering
    \includegraphics[width=\textwidth]{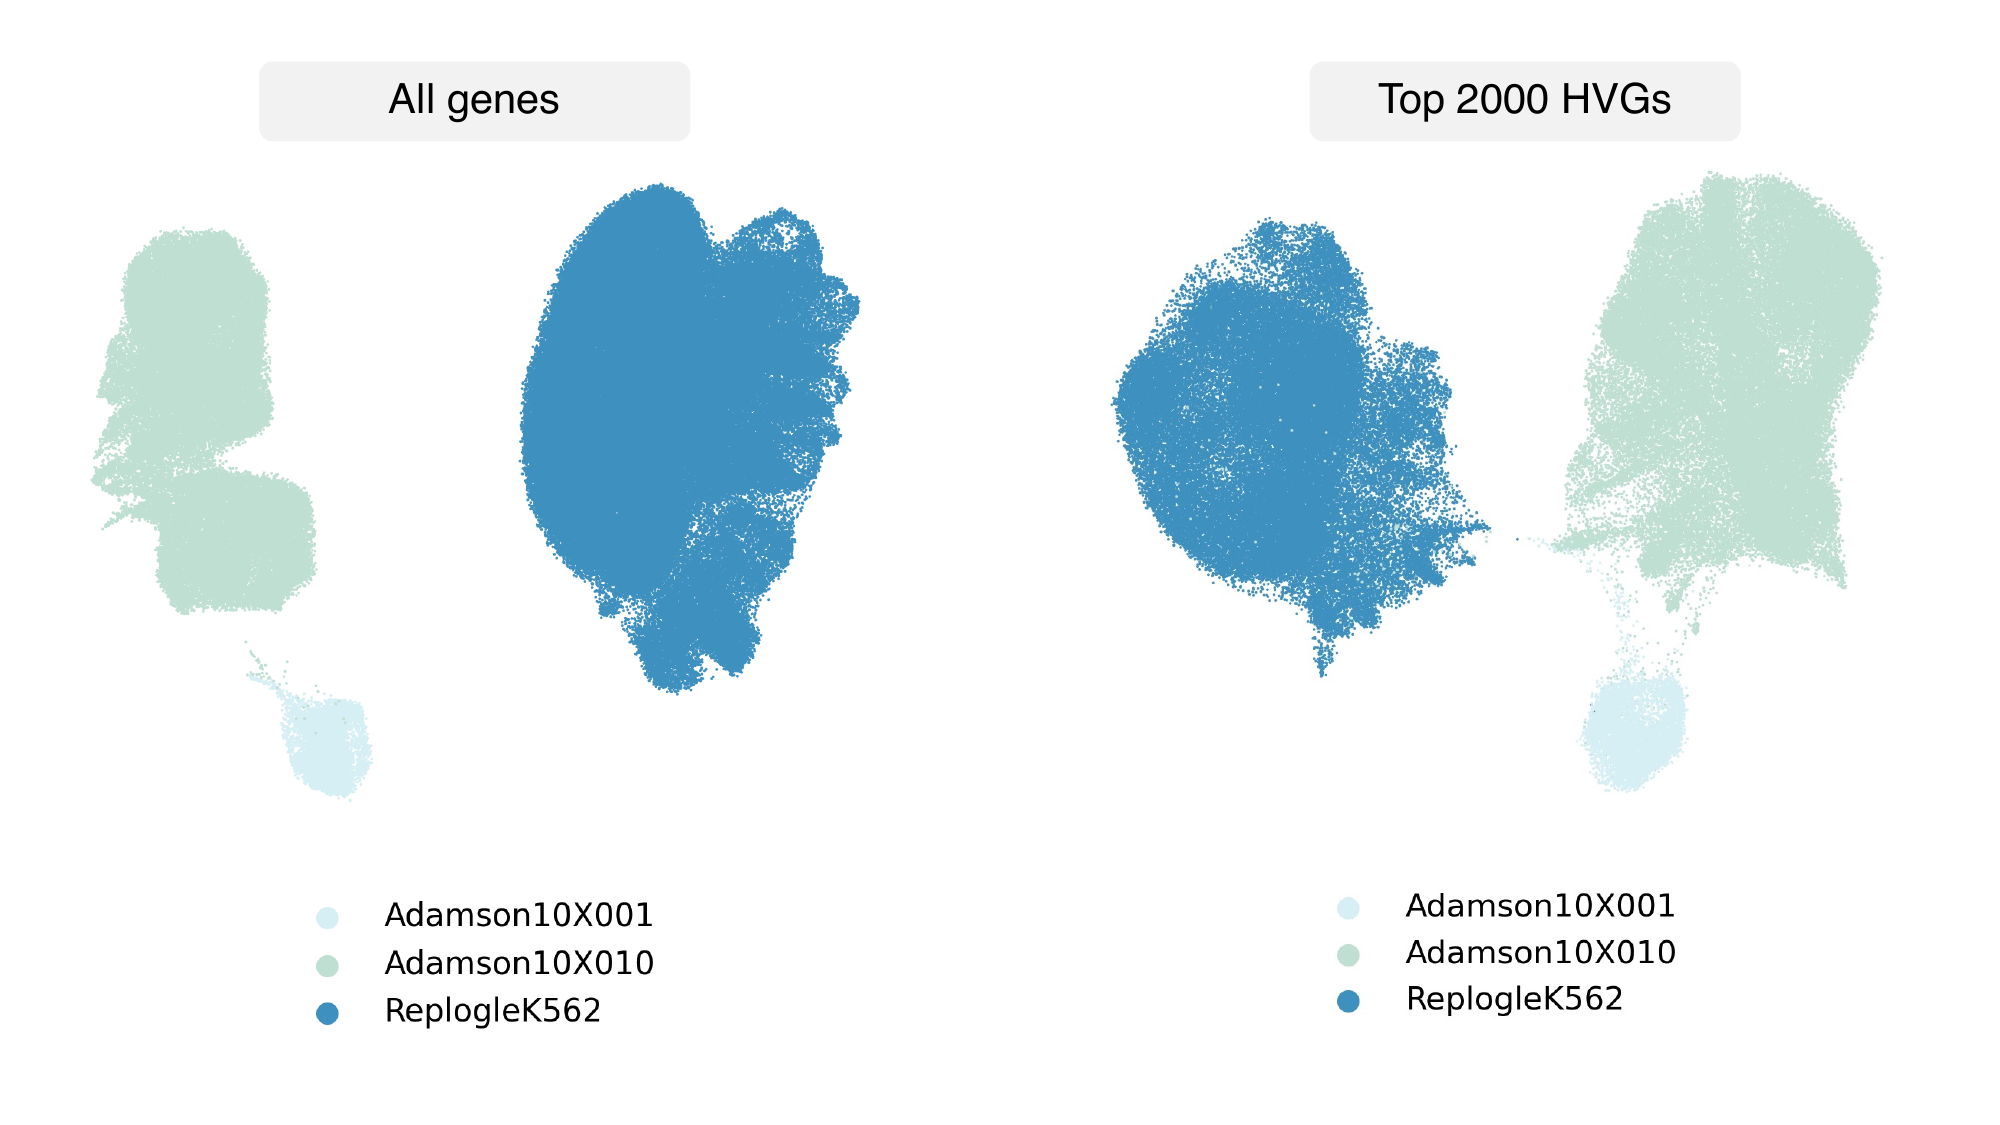}
    \caption{
    \textbf{Effect of feature selection on cross-dataset structure.}
    UMAP visualization of cells from three K562 datasets (Adamson10X001, Adamson10X010, and ReplogleK562) under different feature spaces. UMAP computed using all genes (left) and UMAP computed using the top 2000 highly variable genes (right). 
    }
    \label{fig:umap_hvg_effect}
\end{figure}

\begin{figure}[htbp]
    \centering
    \includegraphics[width=\textwidth]{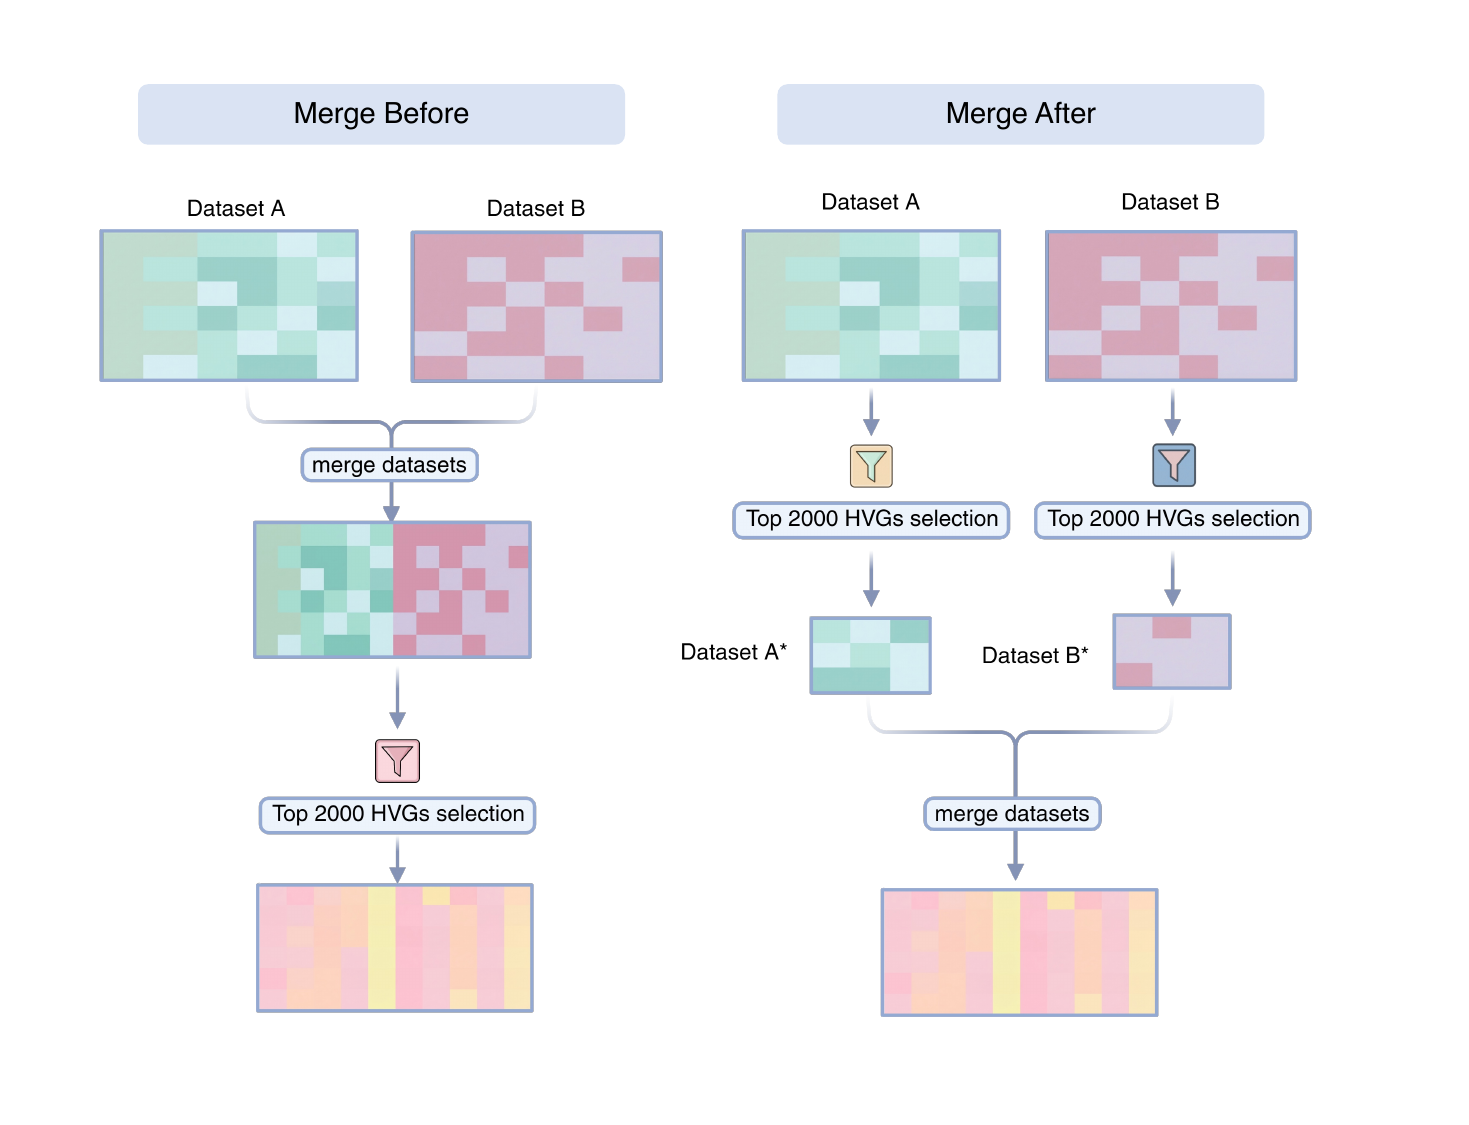}
    \caption{
    \textbf{Illustration of dataset integration strategies.}
    Two alternative pipelines for integrating multiple datasets are shown. In the \emph{merge-before} strategy (left), datasets are concatenated prior to feature selection, and highly variable genes (HVGs) are selected from the merged data. In the \emph{merge-after} strategy (right), HVGs are first selected independently within each dataset, and the resulting feature spaces are then combined during dataset integration.
    }
    \label{fig:merge_strategy}
\end{figure}
